# Supplementary material for: Dataset Condensation with Latent Quantile Matching
Source: arXiv:2406.09860 source file (2024-06-14)
Supplement: Supplementary file 1 [file supp.tex]

% % CVPR 2024 Paper Template; see https://github.com/cvpr-org/author-kit

% \documentclass[10pt,twocolumn,letterpaper]{article}

% %%%%%%%%% PAPER TYPE  - PLEASE UPDATE FOR FINAL VERSION
% \usepackage{cvpr}              % To produce the CAMERA-READY version
% % \usepackage[review]{cvpr}      % To produce the REVIEW version
% % \usepackage[pagenumbers]{cvpr} % To force page numbers, e.g. for an arXiv version

% % Import additional packages in the preamble file, before hyperref
% \input{preamble}

% % It is strongly recommended to use hyperref, especially for the review version.
% % hyperref with option pagebackref eases the reviewers' job.
% % Please disable hyperref *only* if you encounter grave issues, 
% % e.g. with the file validation for the camera-ready version.
% %
% % If you comment hyperref and then uncomment it, you should delete *.aux before re-running LaTeX.
% % (Or just hit 'q' on the first LaTeX run, let it finish, and you should be clear).
% \definecolor{cvprblue}{rgb}{0.21,0.49,0.74}
% \usepackage[pagebackref,breaklinks,colorlinks,citecolor=cvprblue]{hyperref}

% %%%%%%%%% PAPER ID  - PLEASE UPDATE
% \def\paperID{68_13} % *** Enter the Paper ID here
% \def\confName{CVPR}
% \def\confYear{2024}

% %%%%%%%%% TITLE - PLEASE UPDATE
% \title{Appendix of Dataset condensation with latent quantile matching}

% %%%%%%%%% AUTHORS - PLEASE UPDATE
% \author{Wei Wei$^{1}$, Tom De Schepper$^{1}$, Kevin Mets$^{2}$\\
% University of Antwerp - imec, IDLab, \\$^{1}$Department of Computer Science, $^{2}$Faculty of Applied Engineering,\\ Sint-Pietersvliet 7, 2000 Antwerp, Belgium\\
% {\tt\small \{wei.wei, tom.deschepper, kevin.mets\}@uantwerpen.be}
% % For a paper whose authors are all at the same institution,
% % omit the following lines up until the closing ``}''.
% % Additional authors and addresses can be added with ``\and'',
% % just like the second author.
% % To save space, use either the email address or home page, not both
% % Second Author\\
% % Institution2\\
% % First line of institution2 address\\
% % {\tt\small secondauthor@i2.org}
% % \and
% }

% \begin{document}
% \maketitle

% %%%%%%%%%%%%%%%%%%%%%%%%%%%%%%%%%%%%%%%%%%%%%%%%%%%%%%%%%%%%%%%%%%%%%%%%%%%%%%%
% %%%%%%%%%%%%%%%%%%%%%%%%%%%%%%%%%%%%%%%%%%%%%%%%%%%%%%%%%%%%%%%%%%%%%%%%%%%%%%%
% % APPENDIX
% %%%%%%%%%%%%%%%%%%%%%%%%%%%%%%%%%%%%%%%%%%%%%%%%%%%%%%%%%%%%%%%%%%%%%%%%%%%%%%%
% %%%%%%%%%%%%%%%%%%%%%%%%%%%%%%%%%%%%%%%%%%%%%%%%%%%%%%%%%%%%%%%%%%%%%%%%%%%%%%%
% \appendix
% \onecolumn

% \section{Ablation study}\label{section:ablation}
% \textbf{Choices of goodness of fit tests. }
% In \citet{barbiero2023discrete}, the optimal quantiles of the CvM and AD test statistics are reported. The optimal quantiles for AD test statistics can be obtained by an iterative process. We report the process proposed by \citet{barbiero2023discrete} in \cref{sec:ADalgo}. The quantiles obtained will minimize the AD test statistic, which is a variant of the CvM test statistic that gives more weight to the tails of the distribution. We have experimented with the optimal quantiles that minimize the AD test statistic with graph structured data. The result is shown in \cref{tab:ADperf}.

% Compared to the performance of optimal CvM quantiles, the optimal AD quantiles does not provide noticeable improvements across the four experimented dataset. In the one task setting with graph structured data, the variant that uses optimal CvM quantiles consistently outperform the variant that uses optimal AD quantiles. Next, the computation of CvM quantiles does not require an iterative process. Thus, the use of the CvM test is more suitable for DM based DC.

% \begin{table*}[h]
%     \label{tab:ADperf}
% \begin{center}
% \begin{small}
% \begin{sc}

%     \begin{adjustbox}{width=\textwidth, center}
    
%     \begin{tabular}{c|c|cc|cc|cc|cc}
%     \toprule
%     \multirow{2}{*}{Setting} & \multirow{2}{*}{Methods} & \multicolumn{2}{c}{CoraFull} & \multicolumn{2}{c}{Arxiv} & \multicolumn{2}{c}{Reddit} & \multicolumn{2}{c}{Product}\\
%     \cmidrule{3-10}
    
%     &&AA(\%)$\uparrow$ & BWT(\%)$\uparrow$ &AA(\%)$\uparrow$&BWT(\%)$\uparrow$&AA(\%)$\uparrow$&BWT(\%)$\uparrow$&AA(\%)$\uparrow$&BWT(\%)$\uparrow$
%     \\
    
%     \midrule
    
%     \multirow{2}{*}{One task}
%     & CaT+LQM (AD)&
%     57.0±0.2&- &67.2±0.2&- &\textbf{92.8±0.1}&- &84.3±0.1&-\\
%     &CaT+LQM (CvM)&
%     \textbf{57.5±0.2}& -&\textbf{67.6±0.4}& - &\textbf{92.8±0.1}& - &\textbf{84.4±0.1}& - \\


%     \midrule
%     \midrule

%     \multirow{2}{*}{CGL}
%     & CaT+LQM (AD)&
%     \textbf{68.3$\pm$0.4}&\textbf{-8.7$\pm$0.2} &67.1$\pm$0.2&-11.8$\pm$0.6 &\textbf{97.2$\pm$0.1}&\textbf{-0.5$\pm$0.1} &\textbf{71.0$\pm$0.4}&-5.0$\pm$0.3\\
%     &CaT+LQM (CvM)&
%     68.1$\pm$0.2&\textbf{-8.7$\pm$0.3} & \textbf{68.0$\pm$0.3}&\textbf{-10.7$\pm$0.2} &97.1$\pm$0.0&\textbf{-0.5$\pm$0.0} &\textbf{71.0$\pm$0.2}&\textbf{-4.9$\pm$0.2} \\

    
%     \bottomrule
    
%     \end{tabular}
%     \end{adjustbox}
%     \end{sc}
%     \end{small}
%     \end{center}
%     \caption{Comparison of AA of LQM using two different goodness of fit test statistic. The bold results are the best performance. ↑ denotes the greater value represents greater performance.}
% \end{table*}


% \section{Algorithm of optimal quantiles for Anderson-Darling test statistic}\label{sec:ADalgo}
% {
% \setlength{\algomargin}{1.5em}
% \begin{algorithm2e*}
%     \caption{Optimal quantile computation for Anderson-Darling test statistic}\label{alg:ADdistance}
%     \SetKwInOut{Input}{Input}
%     \SetKwInOut{Parameter}{Params}

%     \SetKwInOut{Output}{Output}

%     \Input{Budget of discrete points $k$, epsilon $\epsilon_{max}$ for convergence checking}
%     \Parameter{For $i=\{1,2,...,k\}$: quantile of the target distribution $q_i$, quantile of the discrete approximating distribution $Q_i$, probability of the discrete approximations $p_i$, loop counter $t$.}
%   \BlankLine
%     \BlankLine
%     initialize $t = 1$\\
%     \For{$i = 1$ \KwTo $k$}{
%     initialize $p_{i}^0 = \frac{1}{k}, Q_{i}^0 = \frac{1}{k}.$
%     }
    
%     \While{$\epsilon_t > \epsilon_{max}$}{
%         $t\leftarrow t+1$\\
%         \For{$i = 1$ \KwTo $k$}{
%             $q_{i}^t=\frac{Q_{i-1}^{t-1}+Q_{i}^{t-1}}{2}$\\
%             $Q_{i}^t=log(\frac{1-q_i^t}{1-q_{i+1}^t})/log(\frac{q_{i+1}^t(1-q_i^t)}{q_i^t(1-q_{i+1}^t)})$\\
%             $p_i^t=Q_i^t-Q_{i-1}^t$\\
%         }
%         $\epsilon_t = max_{i=1}^k|p_i^t-p_i^{t-1}|$\\
%     }

%    \Output{Quantiles $q_i$ that minimizes the Anderson-Darling test statistic.}
% \end{algorithm2e*}
% }

% \section{Visualizations of synthetic image datasets learned by IDM+LQM}
% We visualize the synthetic image dataset learned by IDM+LQM from \cref{fig:start} to \cref{fig:end}. We observe some repetitive dot patterns in the synthetic datasets learned in 1 image per setting, i.e., in \cref{fig:cifar1} and \cref{fig:tiny1}. In the corresponding 10 image per class setting for TinyImageNet demonstrated in \cref{fig:end}, this is less severe. This may indicate that in 1 image per class setting, the quantiles can't be matched perfectly if we want to maintain the image details.


% \begin{figure*}
% \includegraphics[width=0.58\textwidth]{figures/cifar10_10.png}
% \centering
% % \captionsetup{justification=centering,margin=0cm}
% \caption{Synthetic image dataset learned by IDM+LQM on CIFAR10 with 10 image per class, each row corresponds to a class.}
% \label{fig:start}
% \end{figure*}

% \begin{figure*}
% \includegraphics[width=0.58\textwidth]{figures/cifar100_1.png}
% \centering
% % \captionsetup{justification=centering,margin=0cm}
% \caption{Synthetic image dataset learned by IDM+LQM on CIFAR100 with 1 image per class.}
% \label{fig:cifar1}
% \end{figure*}

% \begin{figure*}
% \includegraphics[width=0.58\textwidth]{figures/TinyImageNet_1.png}
% \centering
% % \captionsetup{justification=centering,margin=0cm}
% \caption{Synthetic image dataset learned by IDM+LQM on TinyImageNet with 1 image per class. Only the first 100 classes are shown.}
% \label{fig:tiny1}
% \end{figure*}


% \begin{figure*}
% \includegraphics[width=0.58\textwidth]{figures/TinyImageNet_10.png}
% \centering
% % \captionsetup{justification=centering,margin=0cm}
% \caption{Synthetic image dataset learned by IDM+LQM on TinyImageNet with 10 image per class. Only the first 10 classes are shown, each row corresponds to a class.}
% \label{fig:end}
% \end{figure*}

% \clearpage
% {
%     \small
%     \bibliographystyle{ieeenat_fullname}
%     \bibliography{main}
% }
% \end{document}
